# Supplementary material for: The Power of Sound (TPoS): Audio Reactive Video Generation with Stable Diffusion
Source: arXiv:2309.04509 source file (2023-09-08)
Supplement: Supplementary file 1 [file supplementary.tex]

% 개요

% A. Implementation Details
% A-a) Architecture Details
% A-b) Training Details
% A-c) Inference details

% B. User Study Details

% C. Ablation Study

% D. Qualitative Results
% D-a) Comparison to other baselines
% D-b) Additional Qualitative Examples

\section{Implementation Details}\vspace{-2mm}~\label{sec:implementationdetail} \myparagraph{Architecture details of Mapping Module.}
The Mapping Module, denoted as \texttt{MAP} in our main paper, consists of several MLP layers, which consist of Linear-Linear-Dropout-GELU layers. The purpose of this module is to align the audio embeddings with textual prompt in Stable Diffusion~\cite{rombach2022high}. The prompt is converted into a sequence vector via the conditional encoder in Stable Diffusion, which is transformers as CLIP-L/14~\cite{radford2021learning} Text Encoder. Since audio embeddings from the Temporal Attention Module is not sequence-like vectors, we use the Mapping Module to broaden the dimensions like text embeddings (e.g. from \texttt{<SOS>} token to \texttt{<EOS>} token). To achieve this, MSE loss is used to align the audio embeddings (e.g. underwater bubbling sound) with the text sequence embeddings of the audio class (e.g. ``Underwater Bubbling") from CLIP-L/14. Specifically, to obtain sequence-like vectors, the \texttt{<SOS>} token is removed from the text embeddings, which is the same for all prompts. Later, we concatenate the \texttt{<SOS>} token with the converted audio embeddings to feed the audio condition into Stable Diffusion in the inference stage.

\myparagraph{Training details.}
 \vspace{-0.1mm}
Our end-to-end Audio Encoder model is trained using a combination of Adam~\cite{kingma2014adam} optimizer and SGD~\cite{ruder2016overview} optimizer. While the Mapping module is trained with Adam optimizer, the remaining modules are trained with SGD optimizer. We distribute the inputs evenly across 4 NVIDIA GeForce RTX 3090 GPUs and train the entire model for 24 epochs. We use the VGG-sound dataset~\cite{chen2020vggsound} and Landscape~\cite{lee2022eccv} for training our model. The Audio Encoder is trained with hyper parameters such as a learning rate of 0.001, a batch size of 160, a weight decaying parameter of 0.0005, dropout of 0.2 and a momentum of 0.9 for the SGD optimizer. Note that our Audio Encoder has not been further fine-tuned for any specific task or experiment.

\myparagraph{Details of Audio Semantic Guidance.} 
To implement the Audio Semantic Guidance module following SEGA~\cite{brack2022stable}, the semantic difference between the concept-conditioned and unconditioned estimates, denoted as $\psi$, is first scaled (see notations in Section 3.3 of our main paper):

\begin{equation}
    \psi(\mathbf{z}^\delta, \mathbf{c}_p, \mathbf{c}_n)=  \epsilon_{\theta}(\mathbf{z}^{\delta},\mathbf{c}_n) - \epsilon_{\theta}(\mathbf{z}^{\delta}_{\varnothing},\mathbf{c}_\varnothing)
\end{equation}

 Then, the values of the distribution $\mathbf{\psi}$ in the upper and lower tail are used as the dimension that represent the specified concept. Therefore, the location to be changed can be obtained, and it can be expressed as:
\begin{align}
  g_s(\mathbf{\psi}; \sigma_c, \lambda) = \left\{
  \begin{array}{lr}
      \sigma_c, & \text{where } |\psi| \geq \eta_{\lambda}(|\psi|) \\
      0, & \text{otherwise.}
  \end{array}
  \right.
\end{align}
% \begin{equation}    
%   \begin{align}
%       g_s(\mathbf{$\psi$};$\sigma$_c,$\lambda$) = $\left$\{\begin{array}{lr}
%       $\sigma$_c, & \text{where} \left|\psi\right| \geq \eta_{\lambda}($\left$|\psi\right|) \\
%       0, & \text{otherwise.}
%       \end{array}
%   \end{align}
% \end{equation}
%
where $\eta_{\lambda}(\left|\psi\right|)$ indicates the $\lambda$-th percentile of $\mathbf{\psi}$, and $\sigma_c$ decides the intensity of the semantic audio guidance. 

Three hyper parameters, namely $\delta$, $\sigma_c$, and $\lambda$, are required for audio semantic guidance. The parameter $\delta$ controls the degree of preservation of the original prompt. In our experiments, we set $\delta$ between 800 and 950 out when $T=1000$ in order to balance the preservation of the original prompt with the visualization of the effect of audio semantics. The $\sigma_c$ hyper parameter represents the degree of the scale of audio semantics effects and it is set to between 2.5 and 8 in our experiments. Note that the $\sigma_c$ hyper parameter is not related to the areas that need to be changed. Instead, it is related to the $\lambda$ parameters, which is set to between 0.8 and 0.99. We stress that these hyper parameters are fixed in a single video.

% Three hyper parameters, namely $\delta$, $s_c$, and $\psi$, are required for audio semantic guidance. The parameter $\delta$ controls the degree of preservation of the original prompt. Lower values of $\delta$ correspond to a greater preservation of the original prompt and $\delta=T$ means no preservation of the original prompt. In our experiments, we set $\delta$ between 800 and 950 to balance the preservation of the original prompt with the visualization of the effect of audio semantics. The $s_c$ hyper parameter represents the degree of the scale of audio semantics effects. $s_c$ is set to between 2.5 and 8 in our experiments. However, the $s_c$ hyper parameter is not related to the areas that need to be changed. Instead, it is related to the $\psi$ parameters. $\psi$ is a value between 0 and 1, and we set it between 0.8 and 0.99. Note that we did not adjust these hyper parameters when creating a single video. Since the distribution of each data is different, we need to make modifications to the hyper parameters for the purpose of improving the visualization of audio semantics and ensuring that the original prompt remains preserved.

%Higher values of $\delta$ correspond to a greater preservation of the original prompt. 

\myparagraph{Details of Quantitative Experiment.}
We observe that Landscape dataset contains class-imbalanced audio, i.e., a large portion of the dataset is related to the sounds of water. Thus, for a more thorough comparison, we use class-balanced sampling to obtain test sets, which makes the performance of Sound-guided Video Generation~\cite{lee2022eccv} degraded. We provide our analysis in Table~\ref{tab:Comparison}.

\begin{table}[t]
    \centering
    \setlength{\tabcolsep}{6pt}
     
    \caption{Comparison of the quality of generated video frames with Sound2Sight~\cite{chatterjee2020sound2sight} and Sound-guided Video Generation~\cite{lee2022eccv} with different data sampling methods.}\vspace{-.5mm}
    \label{tab:Comparison}
    \resizebox{\linewidth}{!}{
    	   \begin{tabular}{@{}lcccccc}
            \toprule
            &\multicolumn{2}{c}{Sound2Sight~\cite{chatterjee2020sound2sight}}&\multicolumn{2}{c}{Sound-guided~
            \cite{lee2022eccv}} & \multicolumn{2}{c}{Ours} \\\cmidrule{2-7}
            & FVD$\downarrow$ & CLIP$\uparrow$ (t$\leftrightarrow$v)&FVD$\downarrow$ & CLIP$\uparrow$ (t$\leftrightarrow$v)&FVD$\downarrow$ & CLIP$\uparrow$ (t$\leftrightarrow$v)\\\midrule
            Random Sampling~\cite{lee2022eccv} &488.18 &0.2025 & 476.67 & 0.2037 & 462.68&0.2416\\\midrule  
            Class-balanced Sampling & 494.28&0.2164&544.09 &0.1702&421.23&0.2436 \\\bottomrule
        \end{tabular}}%}
\end{table}\vspace{-1mm}

%

% \section{Generating Video Frames with Visual Conditioning}~\label{sec:guidance}
%  \yujin{fixed} As we explain in Section 3.3 in our main paper, the model is able to generate the initial frame from random or manual estimated noise space, where manual estimated noise space can be obtained from visual input. Trained diffusion encoder convert image into corresponding noisy latent space. As shown in Figure~\ref{fig:visual_input} (top), based on guided diffusion, where the model is trained such that the unconditioned prediction is pushed in the direction of the conditioned one, the model iteratively performs adjustments, enforcing or suppressing concepts from text prompt and audio semantics, thus steering the overall semantics in diffusion latent space. Figure~\ref{fig:visual_input} (bottom) demonstrates our framework leverages latent space of diffusion model with visual input, text prompt and audio sound.

% \begin{figure}[t]
% \begin{center}
% \includegraphics[width=.9\linewidth]{images/guidance2.pdf} %
%   \caption{A overview of Audio Semantic Guidance Module with visual conditioning. We generate image frame with random visual input, text prompt and audio sound (see bottom).}\vspace{-3mm}
%   \label{fig:visual_input}
% \end{center}
% \end{figure}\vspace{-2mm}

\section{User Study Details}\vspace{-2mm}~\label{sec:userstudydetail}
In user study, participants rate the realness, vividness, consistency of movement, and relevance between audio and video on a five-point scale, ranging from ``1 - very unrealistic'' to ``5 - very realistic,'' ``1 - very unvivid'' to ``5 - very vivid,'' ``1 - very inconsistent'' to ``5 - very consistent," and ``1 - very irrelevant" to ``5 - very relevant,'' respectively. 

Specifically, we ask participants ``On a scale of 1 to 5, how realistic the video is? Please rate the realism, with 1 being very unrealistic and 5 being very realistic'', ``On a scale of 1 to 5, how vibrant does the video appear? Please rate the vividness, with 1 being not vibrant at all and 5 being extremely vibrant.'', ``On a scale of 1 to 5, how well does the movement in the video match the audio levels? Please rate the consistency, with 1 being very inconsistent and 5 being very consistent.'', and ``On a scale of 1 to 5, how relevant video with the audio sound? Please rate the relevance, with 1 being not relevant and 5 being very relevant.''. The order of videos within each question is randomized to prevent participants from inferring the unique quality of each baseline. 

\section{Qualitative Results} \vspace{-2mm} ~\label{sec:morequalitative}

\myparagraph{Comparison to StyleGAN-based baselines.}
We compare our methods with StyleGAN~\cite{karras2021alias} based Tr\"aumerAI~\cite{jeong2021traumerai} and Sound Guided Video Generation~\cite{lee2022eccv} in Figure~\ref{fig:vsstylegan}. StyleGAN based methods both face challenges in effectively aligning audio semantics with latent space of StyleGAN despite of fine-tuning. On the contrary, our model can express the audio semantic meanings in multiple domains thanks to the rich latent space of Stable Diffusion models. Furthermore, compared to other baselines, our model is able to manipulate certain areas (e.g. fire on the stove top) via Audio Semantic Guidance through multiple denoising steps in Stable Diffusion. Our experiment reveals that our method can generate videos that have significant relevance and consistency with audio sound.
 
% We have evaluated the effectiveness of our Audio Encoder in capturing audio semantics by comparing it with other audio-driven video methods. Specifically, we compare it with the recent audio encoder proposed by Lee \etal~\cite{lee2022eccv}. Our analysis shows that our Audio Encoder outperforms other methods in capturing audio semantics, as demonstrated by the improved separation of different classes in the t-sne~\cite{van2008visualizing} plot, as shown in Figure~\ref{}. This improved separation of different classes indicates that our Audio Encoder has a greater ability to distinguish between different semantic meanings present in the audio input. As a result, it is better equipped to manipulate images based on the audio semantics, resulting in a more accurate representation of the audio input in the generated video frames.

% \myparagraph{Text-Audio Joint Conditioning.}
% As our model is built upon the Stable Diffusion model, it is also possible to use text and audio as a condition together. In Figure~\ref{fig:application}, we provide an example where we generate video frames conditioned on a sound of an explosion along with texts, such as ``eruption'', ``spew'', or ``cloud of ash.'' (see 2nd-4th rows) Preserving temporal semantics, our model successfully generates video frames guided by text as well.

\myparagraph{Additional Qualitative Examples.}
 Figure~\ref{fig:water} shows our model can generate video frames in diverse domains. Furthermore, Figure~\ref{fig:same_seed} and Figure~\ref{fig:same_prompt} demonstrate the semantic consistency between sound and video. Lastly, our model can generate multiple high-fidelity frames naturally by the interpolation in Figure~\ref{fig:long_sequence}. %Lastly, We further provide the whole sequences of video frame in Figure~\ref{fig:video1} and Figure~\ref{fig:video2} at fps 15 ~\yujin{need to be fixed}. %It is important to note that we did not conduct any additional training on our Audio Encoder or Stable Diffusion. %\yujin{if we get the results from Figure 6, I need to add @yujin}

% \begin{figure*}
% \begin{center}
% \includegraphics[width=0.72\linewidth]{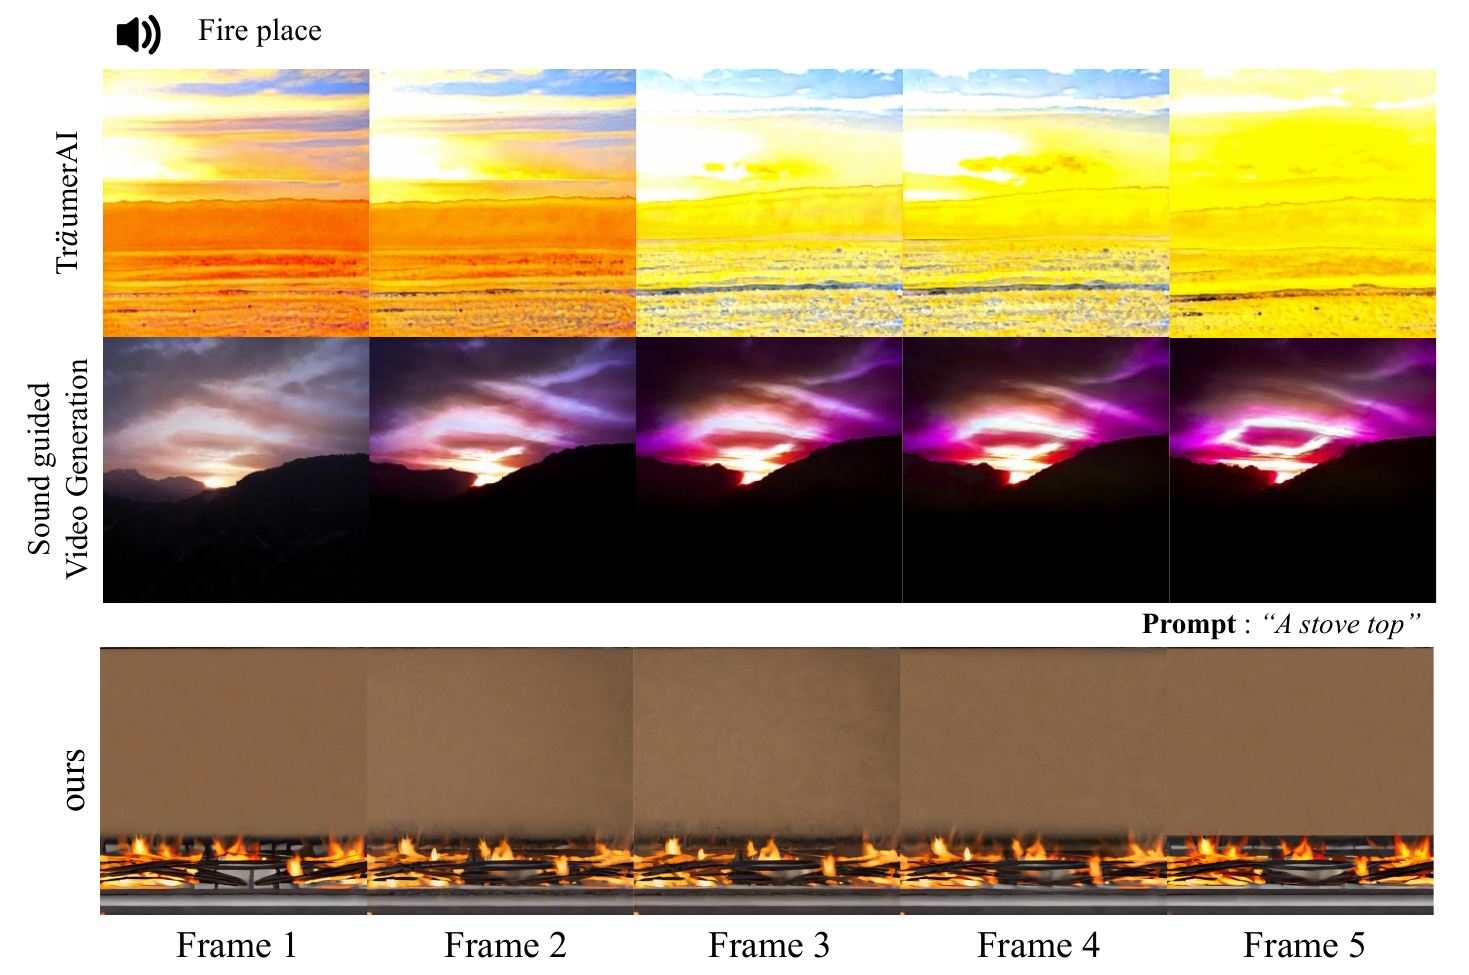} %
%   \caption{Comparison with StyleGAN~\cite{skorokhodov2022stylegan}-based method. First row and second row represent video frames from Tr\"aumerAI~\cite{jeong2021traumerai} and Sound guided Video Generation~\cite{lee2022eccv}. The last row shows video frames which are generated from our model.}
%   \label{fig:vsstylegan}
%   \vspace{-2em}
% \end{center}
% \end{figure*}

% \begin{figure}[t]
% \begin{center}
% \includegraphics[width=\linewidth]{images/vsStyleGAN_sup.pdf} %
%   \caption{Comparison with StyleGAN~\cite{skorokhodov2022stylegan}-based method. First row and second row represent video frames from Tr\"aumerAI~\cite{jeong2021traumerai} and Sound guided Video Generation~\cite{lee2022eccv}. The last row shows video frames which are generated from our model.}
%   \label{fig:vsstylegan}
% \end{center}
% \end{figure}
\begin{figure}
  \centering
  \includegraphics[width=\linewidth]{images/vsStyleGAN_sup.pdf}
  \caption{Comparison with StyleGAN~\cite{skorokhodov2022stylegan}-based method. First row and second row represent video frames from Tr\"aumerAI~\cite{jeong2021traumerai} and Sound guided Video Generation~\cite{lee2022eccv}. The last row shows video frames which are generated from our model.}
  \label{fig:vsstylegan}
\end{figure}

% \begin{figure*}
% \begin{center}
%       \includegraphics[width=.8\linewidth]{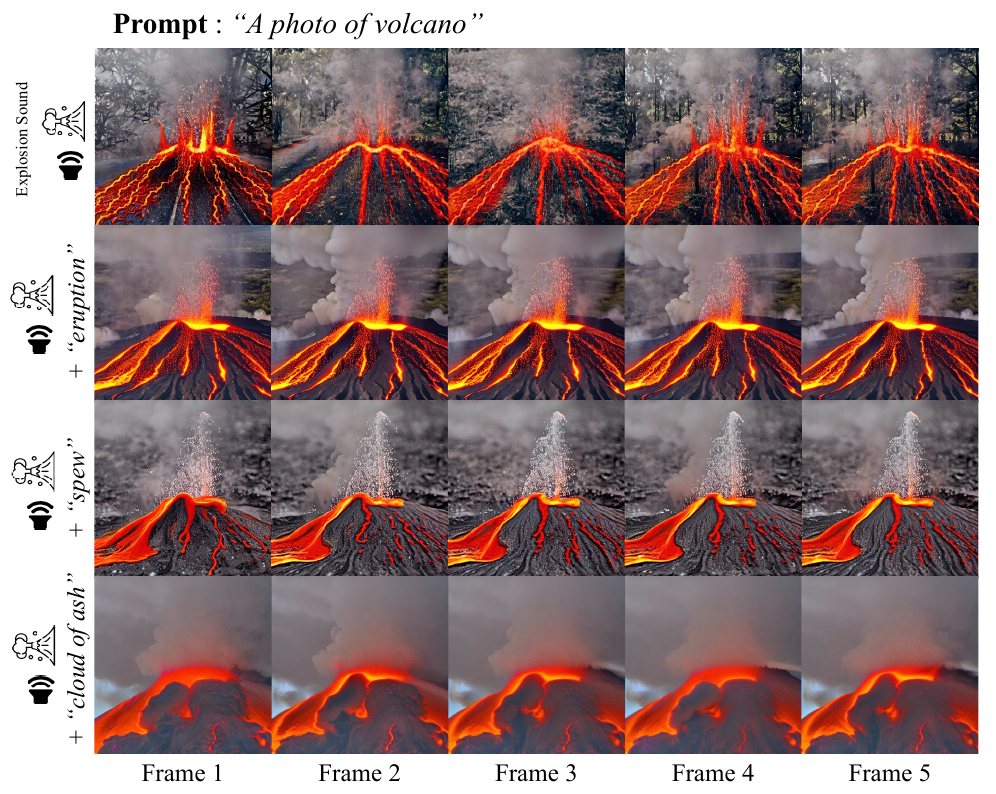} %
%   \caption{Example of generated videos with audio-text joint condition (e.g., 2nd row: conditioned with text ``eruption'' and explosion sound)}
%   \label{fig:application}
%   \vspace{-2em}
% \end{center}
% \end{figure*}

% \begin{figure*}
% \begin{center}
% \includegraphics[width=0.8\linewidth]{images/face.pdf} %
%   \caption{Examples of face generation with our methods. The sound of giggling and sobbing are used.}
%   \label{fig:face}
%   \vspace{-2em}
% \end{center}
% \end{figure*}

\begin{figure*}
\begin{center}
\includegraphics[width=.85\linewidth]{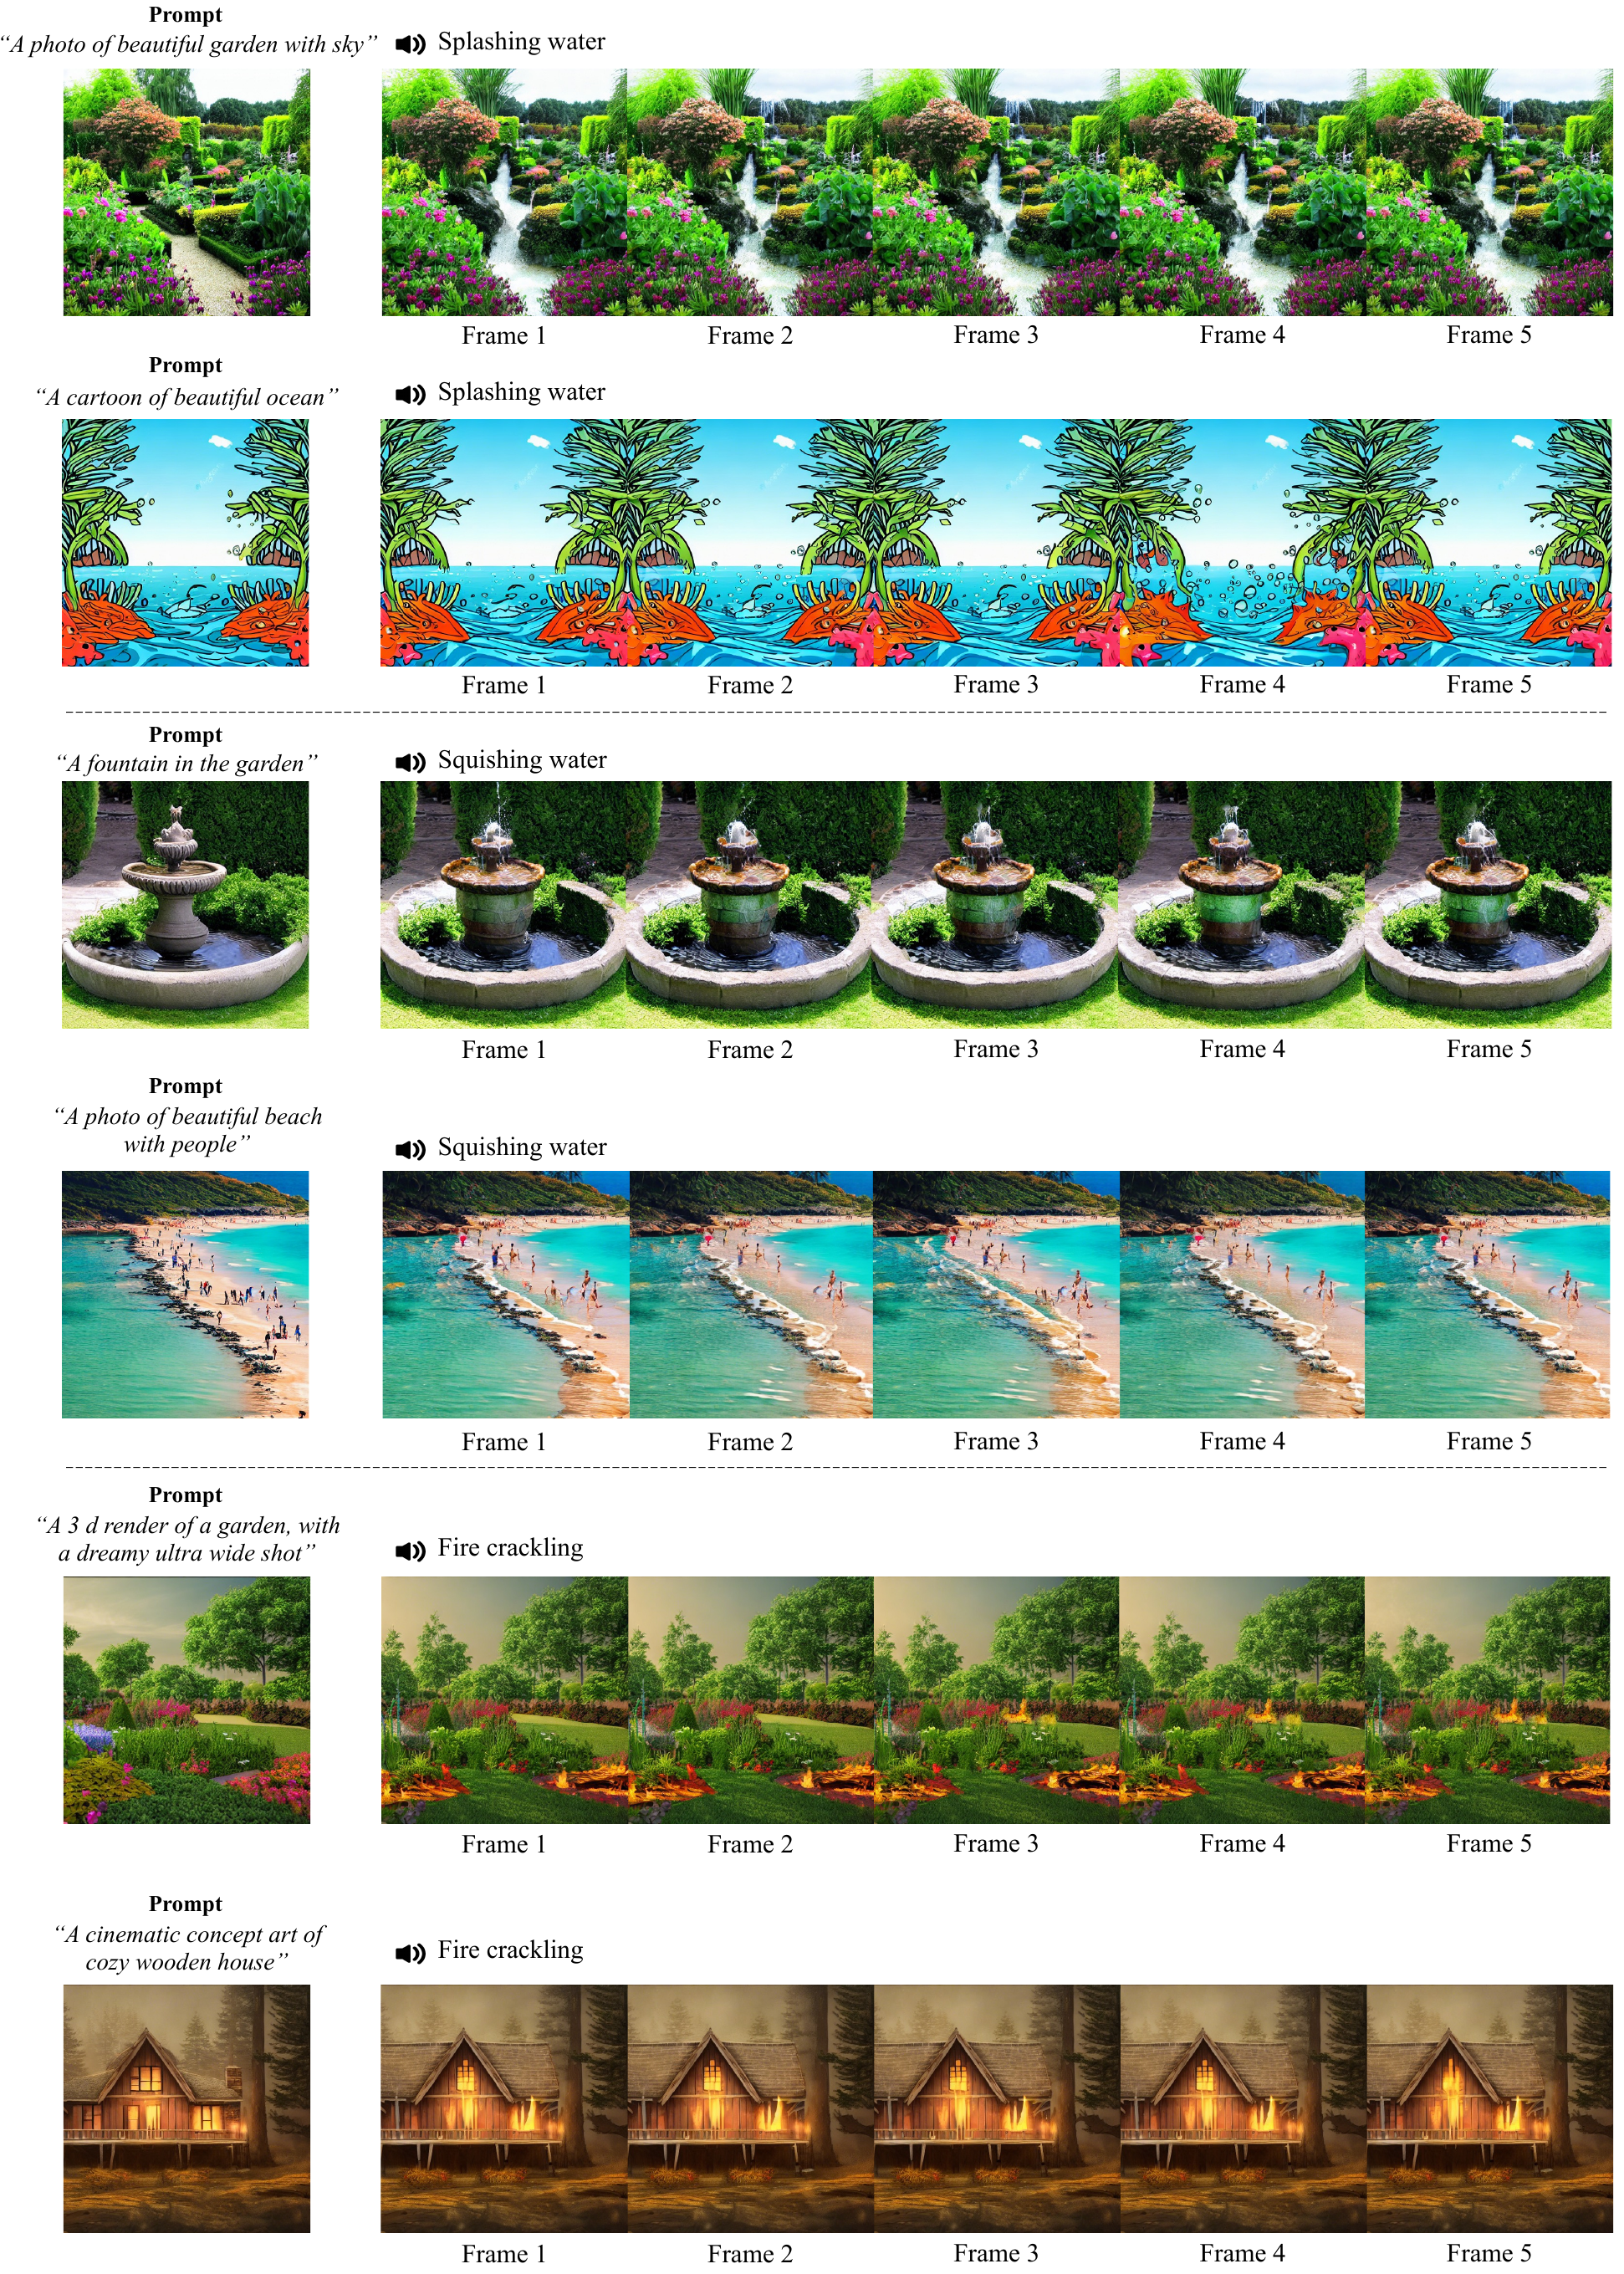} %
  \caption{Examples of diverse examples in open domains. The sound of splashing water, squishing water and fire crackling are used.}
  \label{fig:water}
  \vspace{-5mm}
\end{center}
\end{figure*}

\begin{figure*}
\begin{center}
\includegraphics[width=\linewidth]{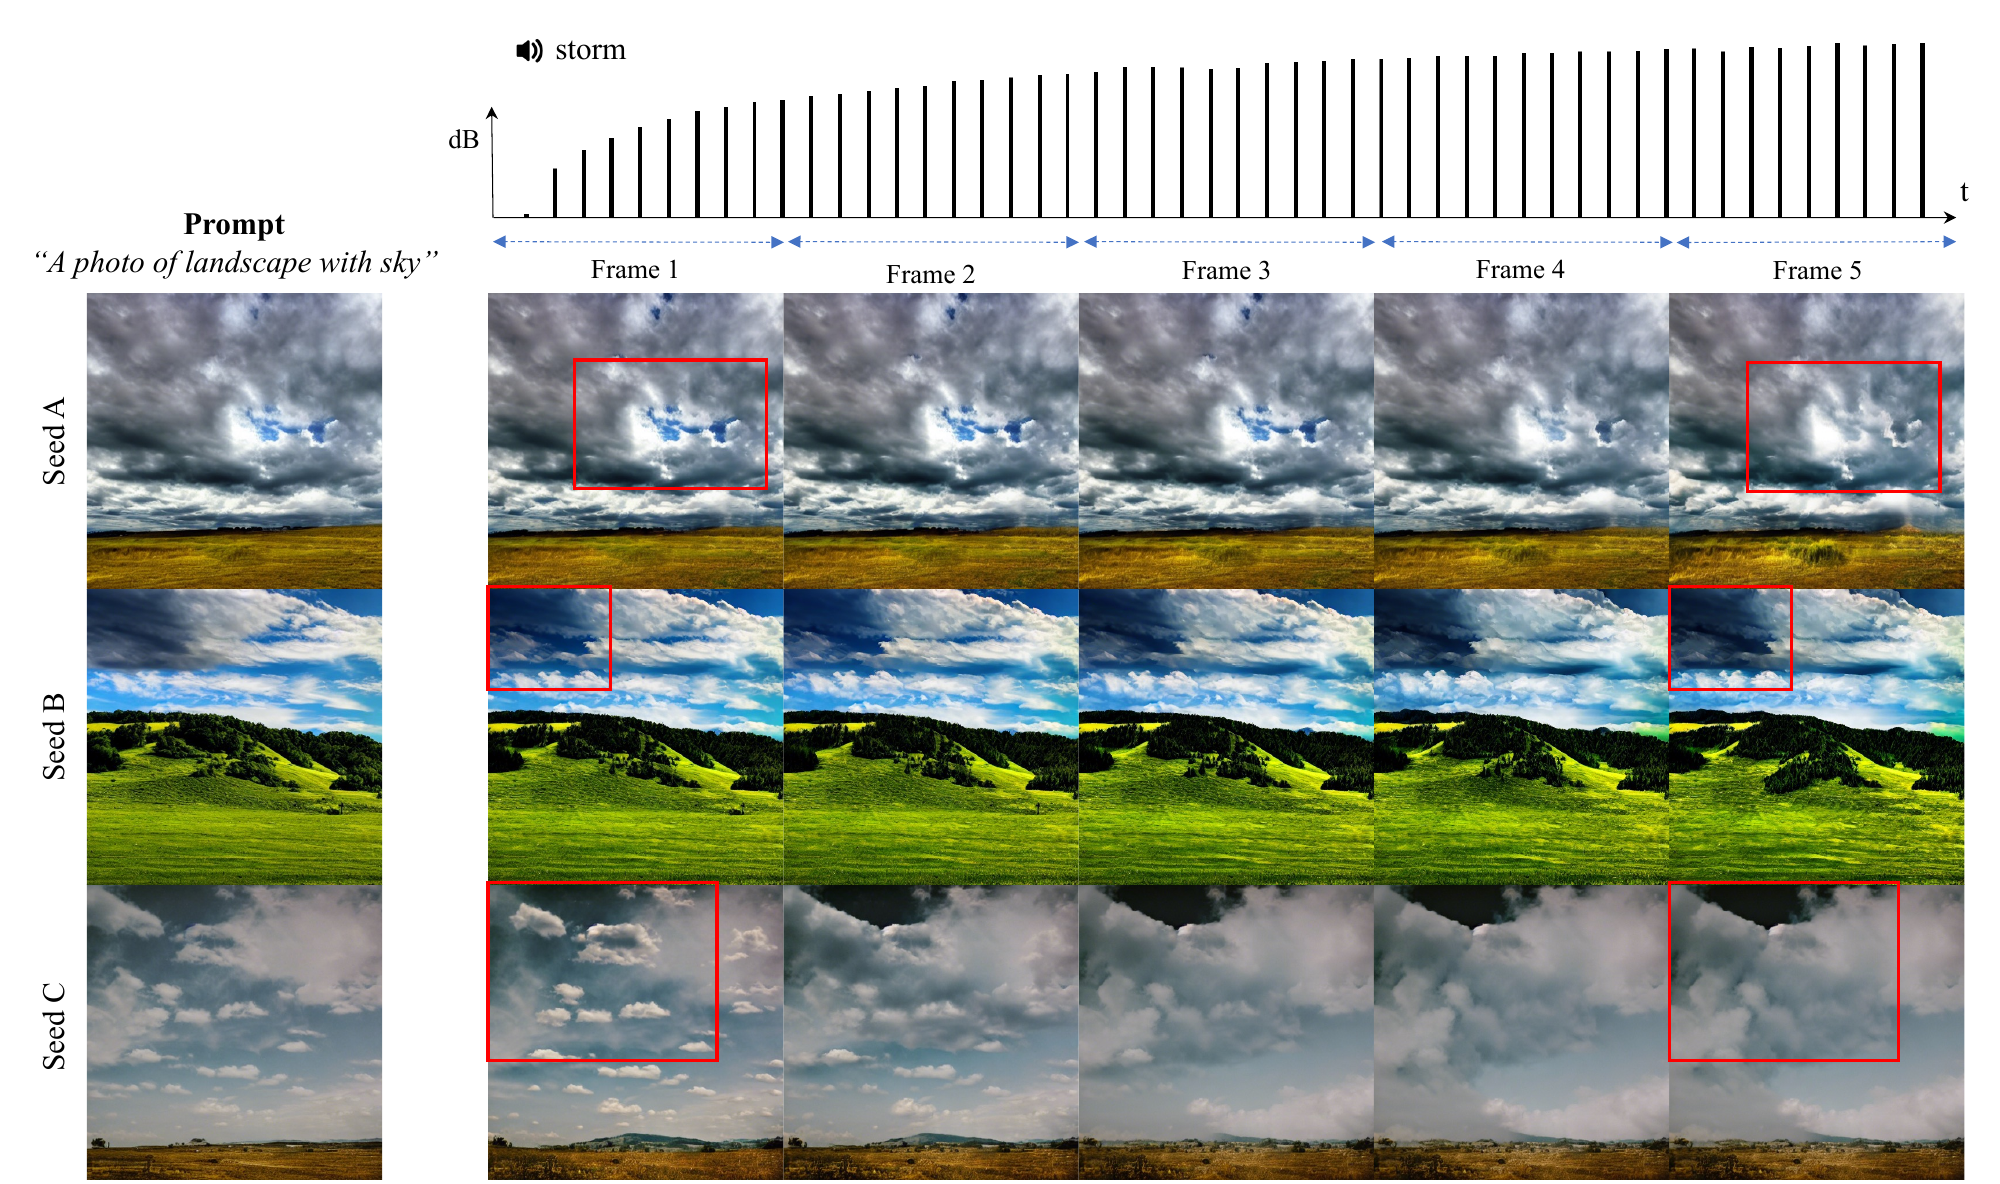} %
  \caption{Example of video frames with multiple seed numbers. We regulate the prompt and audio sound as a given input feature and change a seed number randomly. The video frames are temporally consistent with the magnitude of audio.}
  \label{fig:same_seed}
  \vspace{-5mm}
\end{center}
\end{figure*}

\begin{figure*}
\begin{center}
\includegraphics[width=\linewidth]{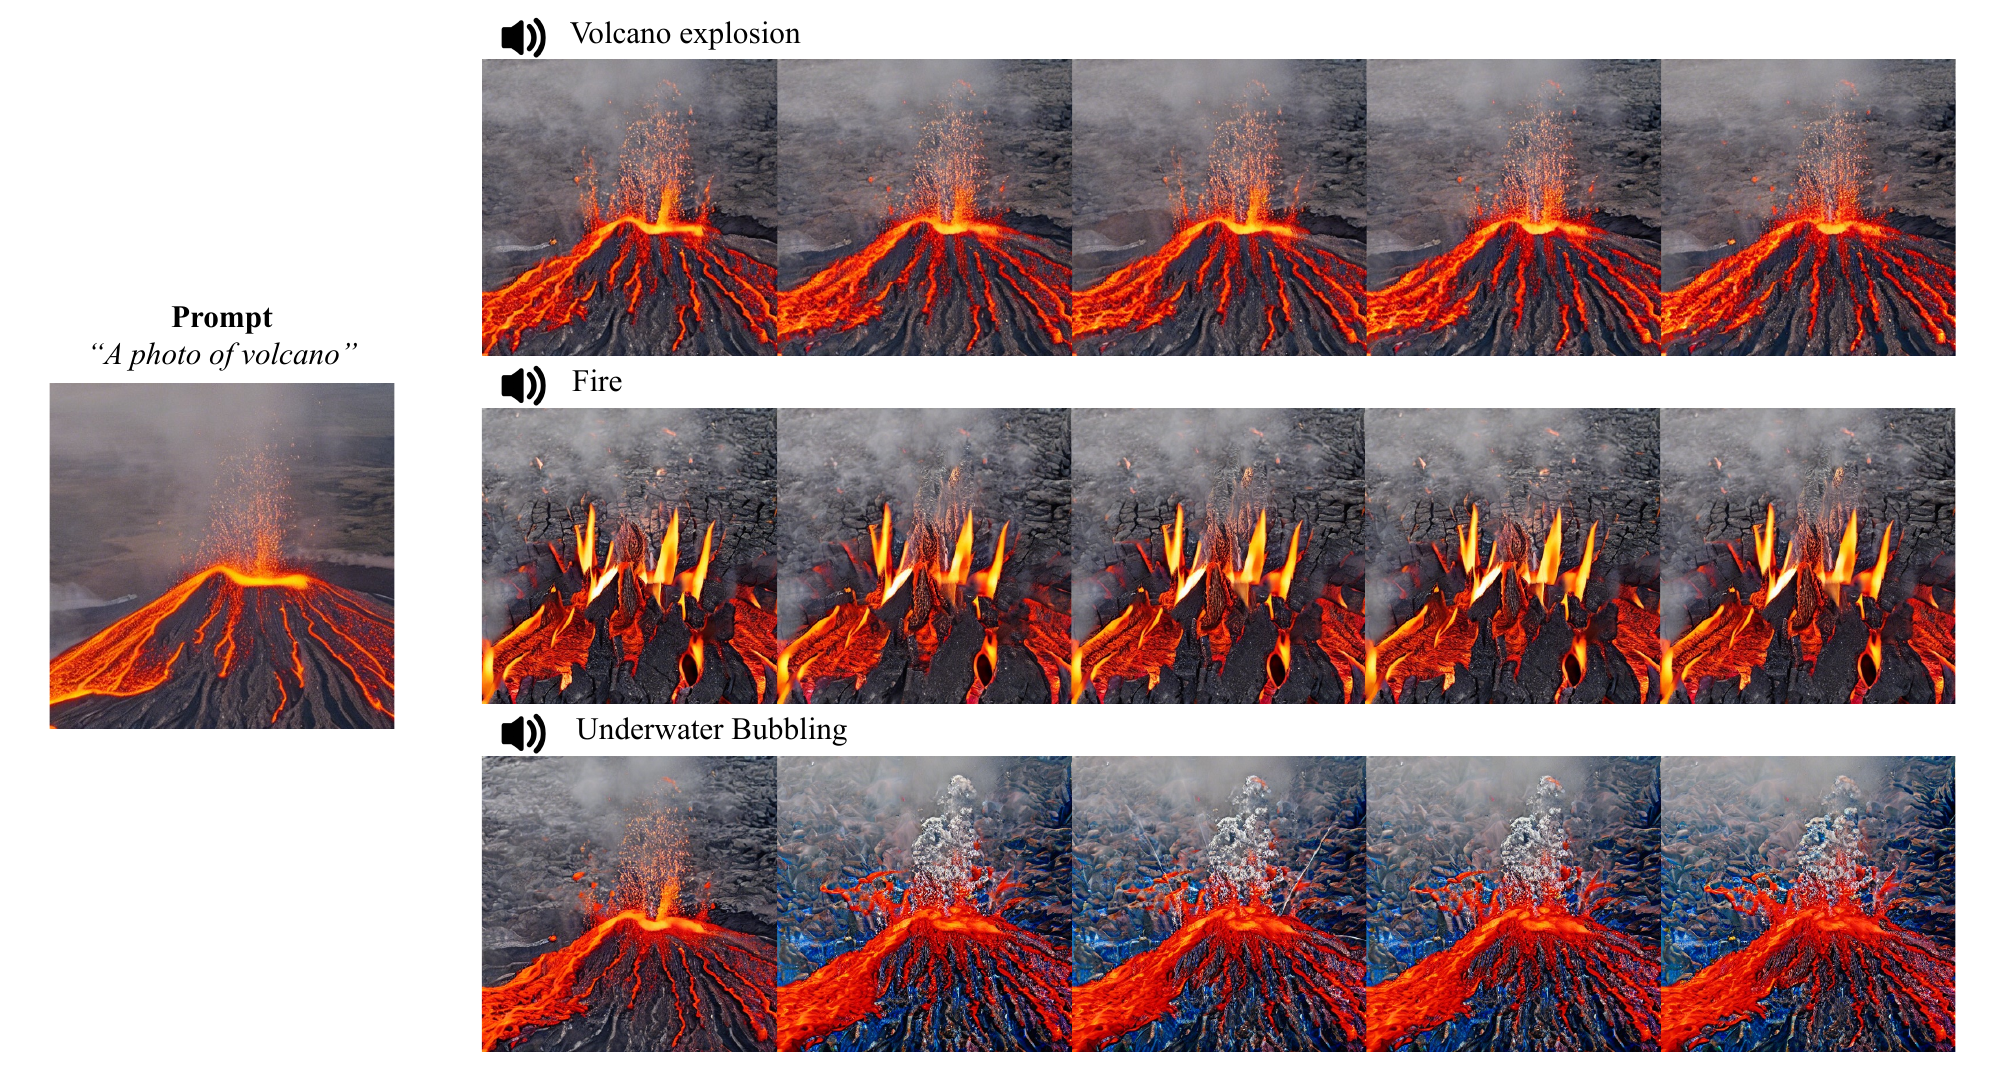} %
  \caption{Example of video frames with different sound. The video frames are consistent and relevant with the audio semantics.}
  \label{fig:same_prompt}
  \vspace{-5mm}
\end{center}
\end{figure*}

\begin{figure*}
\begin{center}
\includegraphics[width=.8\linewidth]{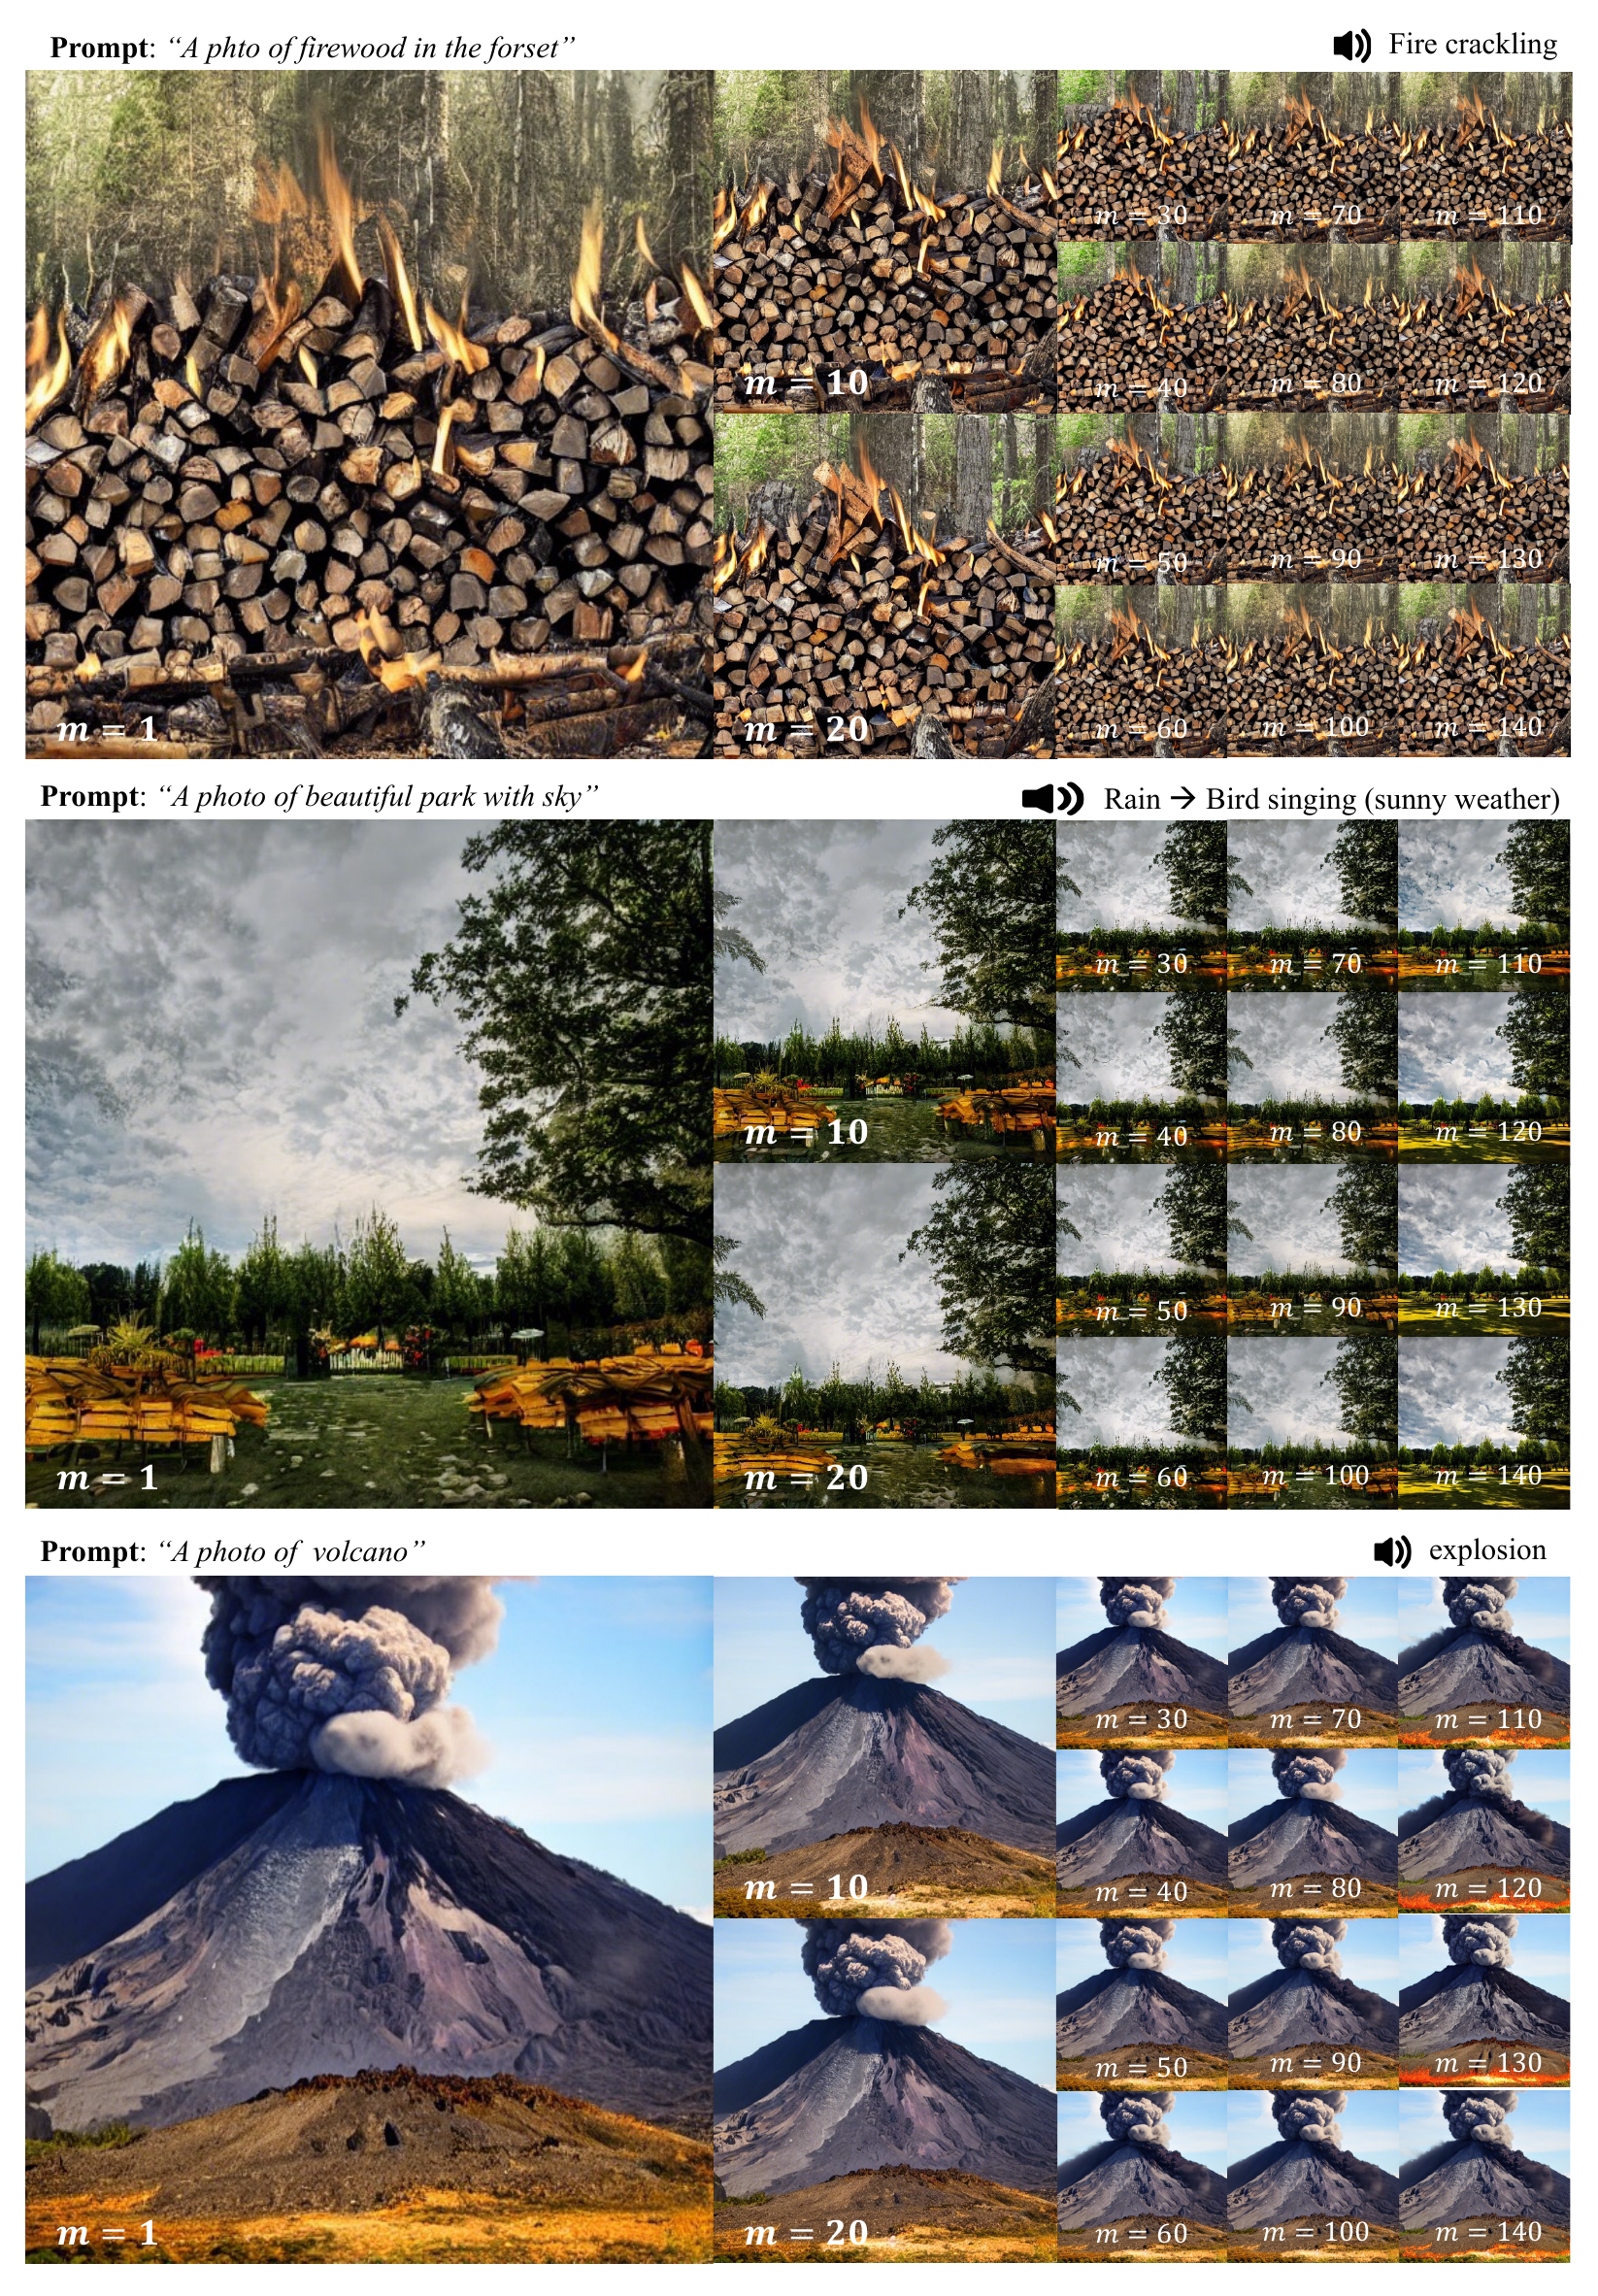} %
  \caption{Example of video frames with interpolation module. A number of video frames are generated reactively by audio sound.}
  \label{fig:long_sequence}
  \vspace{-5mm}
\end{center}
\end{figure*}

% \begin{figure*}
% \begin{center}
% \includegraphics[width=.8\linewidth]{images/video_examples_change.pdf} %
%   \caption{Whole sequence of video frames conditioned by the sound that has a semantic change from wave to fire place. }
%   \label{fig:video1}
%   \vspace{-5mm}
% \end{center}
% \end{figure*}

% \begin{figure*}
% \begin{center}
% \includegraphics[width=.8\linewidth]{images/video_examples_explosion.pdf} %
%   \caption{Whole sequence of video frames conditioned by the sound of explosion}
%   \label{fig:video2}
%   \vspace{-5mm}
% \end{center}
% \end{figure*}

% \clearpage
