# Supplementary material for: The Power of Sound (TPoS): Audio Reactive Video Generation with Stable Diffusion
Source: arXiv:2309.04509 source file (2023-09-08)
Supplement: Supplementary file 2 [file 07327-supp.pdf]

# Supplemental Materials to The Power of Sound (TPoS): Audio Reactive Video Generation with Stable Diffusion

Yujin Jeong<sup>1</sup>, Wonjeong Ryoo<sup>2</sup>, Seunghyun Lee<sup>2</sup>, Dabin Seo<sup>1</sup>,  
Wonmin Byeon<sup>3</sup>, Sangpil Kim,<sup>2,\*</sup> and Jinkyu Kim<sup>1,\*</sup>

<sup>1</sup> Department of Computer Science and Engineering, Korea University, Seoul 02841, Korea

<sup>2</sup> Department of Artificial Intelligence, Korea University, Seoul 02841, Korea

<sup>3</sup> NVIDIA Research, Santa Clara 95050, USA

\*Correspondences: S. Kim (spk7@korea.ac.kr) and J. Kim (jinkyukim@korea.ac.kr)

## Overview

*This supplementary material provides implementation details including the architecture details, training details and inference details of The Power of Sound (TPoS) in Section A. Next, in Section B, we provide our detailed survey methods and analysis of user study. Finally, in Section C, we show a wider range of qualitative results in two ways: (i) comparison to StyleGAN [5]-based audio-driven video methods, and (ii) demonstrating multiple examples in an open domain.*

## A. Implementation Details

**Architecture details of Mapping Module.** The Mapping Module, denoted as MAP in our main paper, consists of several MLP layers, which consist of Linear-Linear-Dropout-GELU layers. The purpose of this module is to align the audio embeddings with textual prompt in Stable Diffusion [9]. The prompt is converted into a sequence vector via the conditional encoder in Stable Diffusion, which is transformers as CLIP-L/14 [8] Text Encoder. Since audio embeddings from the Temporal Attention Module is not sequence-like vectors, we use the Mapping Module to broaden the dimensions like text embeddings (e.g. from <SOS> token to <EOS> token). To achieve this, MSE loss is used to align the audio embeddings (e.g. underwater bubbling sound) with the text sequence embeddings of the audio class (e.g. “Underwater Bubbling”) from CLIP-L/14. Specifically, to obtain sequence-like vectors, the <SOS> token is removed from the text embeddings, which is the same for all prompts. Later, we concatenate the <SOS> token with the converted audio embeddings to feed the audio condition into Stable Diffusion in the inference stage.

**Training details.** Our end-to-end Audio Encoder model

is trained using a combination of Adam [6] optimizer and SGD [10] optimizer. While the Mapping module is trained with Adam optimizer, the remaining modules are trained with SGD optimizer. We distribute the inputs evenly across 4 NVIDIA GeForce RTX 3090 GPUs and train the entire model for 24 epochs. We use the VGG-sound dataset [3] and Landscape [7] for training our model. The Audio Encoder is trained with hyper parameters such as a learning rate of 0.001, a batch size of 160, a weight decaying parameter of 0.0005, dropout of 0.2 and a momentum of 0.9 for the SGD optimizer. Note that our Audio Encoder has not been further fine-tuned for any specific task or experiment.

**Details of Audio Semantic Guidance.** To implement the Audio Semantic Guidance module following SEGA [1], the semantic difference between the concept-conditioned and unconditioned estimates, denoted as  $\psi$ , is first scaled (see notations in Section 3.3 of our main paper):

$$\psi(\mathbf{z}^\delta, \mathbf{c}_p, \mathbf{c}_n) = \epsilon_\theta(\mathbf{z}^\delta, \mathbf{c}_n) - \epsilon_\theta(\mathbf{z}^\delta, \mathbf{c}_\emptyset) \quad (1)$$

Then, the values of the distribution  $\psi$  in the upper and lower tail are used as the dimension that represent the specified concept. Therefore, the location to be changed can be obtained, and it can be expressed as:

$$g_s(\psi; \sigma_c, \lambda) = \begin{cases} \sigma_c, & \text{where } |\psi| \geq \eta_\lambda(|\psi|) \\ 0, & \text{otherwise.} \end{cases} \quad (2)$$

where  $\eta_\lambda(|\psi|)$  indicates the  $\lambda$ -th percentile of  $\psi$ , and  $\sigma_c$  decides the intensity of the semantic audio guidance.

Three hyper parameters, namely  $\delta$ ,  $\sigma_c$ , and  $\lambda$ , are required for audio semantic guidance. The parameter  $\delta$  controls the degree of preservation of the original prompt. In our experiments, we set  $\delta$  between 800 and 950 out when  $T = 1000$  in order to balance the preservation of the original prompt with the visualization of the effect of audio se-

Table 1: Comparison of the quality of generated video frames with Sound2Sight [2] and Sound-guided Video Generation [7] with different data sampling methods.

|                         | Sound2Sight [2] |             | Sound-guided [7] |             | Ours   |             |
|-------------------------|-----------------|-------------|------------------|-------------|--------|-------------|
|                         | FVD↓            | CLIP↑ (t→v) | FVD↓             | CLIP↑ (t→v) | FVD↓   | CLIP↑ (t→v) |
| Random Sampling [7]     | 488.18          | 0.2025      | 476.67           | 0.2037      | 462.68 | 0.2416      |
| Class-balanced Sampling | 494.28          | 0.2164      | 544.09           | 0.1702      | 421.23 | 0.2436      |

manatics. The  $\sigma_c$  hyper parameter represents the degree of the scale of audio semantics effects and it is set to between 2.5 and 8 in our experiments. Note that the  $\sigma_c$  hyper parameter is not related to the areas that need to be changed. Instead, it is related to the  $\lambda$  parameters, which is set to between 0.8 and 0.99. We stress that these hyper parameters are fixed in a single video.

**Details of Quantitative Experiment.** We observe that Landscape dataset contains class-imbalanced audio, i.e., a large portion of the dataset is related to the sounds of water. Thus, for a more thorough comparison, we use class-balanced sampling to obtain test sets, which makes the performance of Sound-guided Video Generation [7] degraded. We provide our analysis in Table 1.

## B. User Study Details

In user study, participants rate the realness, vividness, consistency of movement, and relevance between audio and video on a five-point scale, ranging from “1 - very unrealistic” to “5 - very realistic,” “1 - very unvivid” to “5 - very vivid,” “1 - very inconsistent” to “5 - very consistent,” and “1 - very irrelevant” to “5 - very relevant,” respectively.

Specifically, we ask participants “On a scale of 1 to 5, how realistic the video is? Please rate the realism, with 1 being very unrealistic and 5 being very realistic”, “On a scale of 1 to 5, how vibrant does the video appear? Please rate the vividness, with 1 being not vibrant at all and 5 being extremely vibrant.”, “On a scale of 1 to 5, how well does the movement in the video match the audio levels? Please rate the consistency, with 1 being very inconsistent and 5 being very consistent.”, and “On a scale of 1 to 5, how relevant video with the audio sound? Please rate the relevance, with 1 being not relevant and 5 being very relevant.”. The order of videos within each question is randomized to prevent participants from inferring the unique quality of each baseline.

## C. Qualitative Results

**Comparison to StyleGAN-based baselines.** We compare our methods with StyleGAN [5] based TrumerAI [4] and Sound Guided Video Generation [7] in Figure 1. StyleGAN based methods both face challenges in effectively aligning

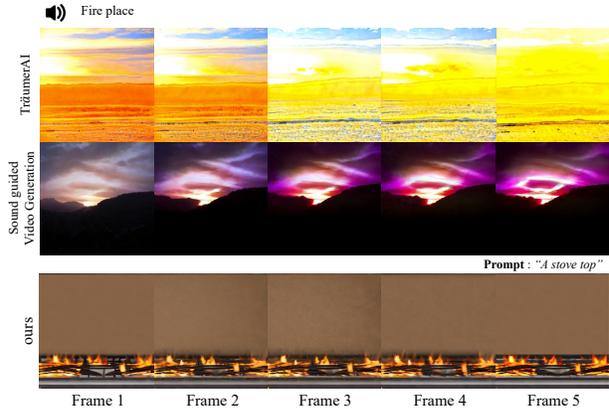

Figure 1: Comparison with StyleGAN [11]-based method. First row and second row represent video frames from TrumerAI [4] and Sound guided Video Generation [7]. The last row shows video frames which are generated from our model.

audio semantics with latent space of StyleGAN despite of fine-tuning. On the contrary, our model can express the audio semantic meanings in multiple domains thanks to the rich latent space of Stable Diffusion models. Furthermore, compared to other baselines, our model is able to manipulate certain areas (e.g. fire on the stove top) via Audio Semantic Guidance through multiple denoising steps in Stable Diffusion. Our experiment reveals that our method can generate videos that have significant relevance and consistency with audio sound.

**Additional Qualitative Examples.** Figure 2 shows our model can generate video frames in diverse domains. Furthermore, Figure 3 and Figure 4 demonstrate the semantic consistency between sound and video. Lastly, our model can generate multiple high-fidelity frames naturally by the interpolation in Figure 5.

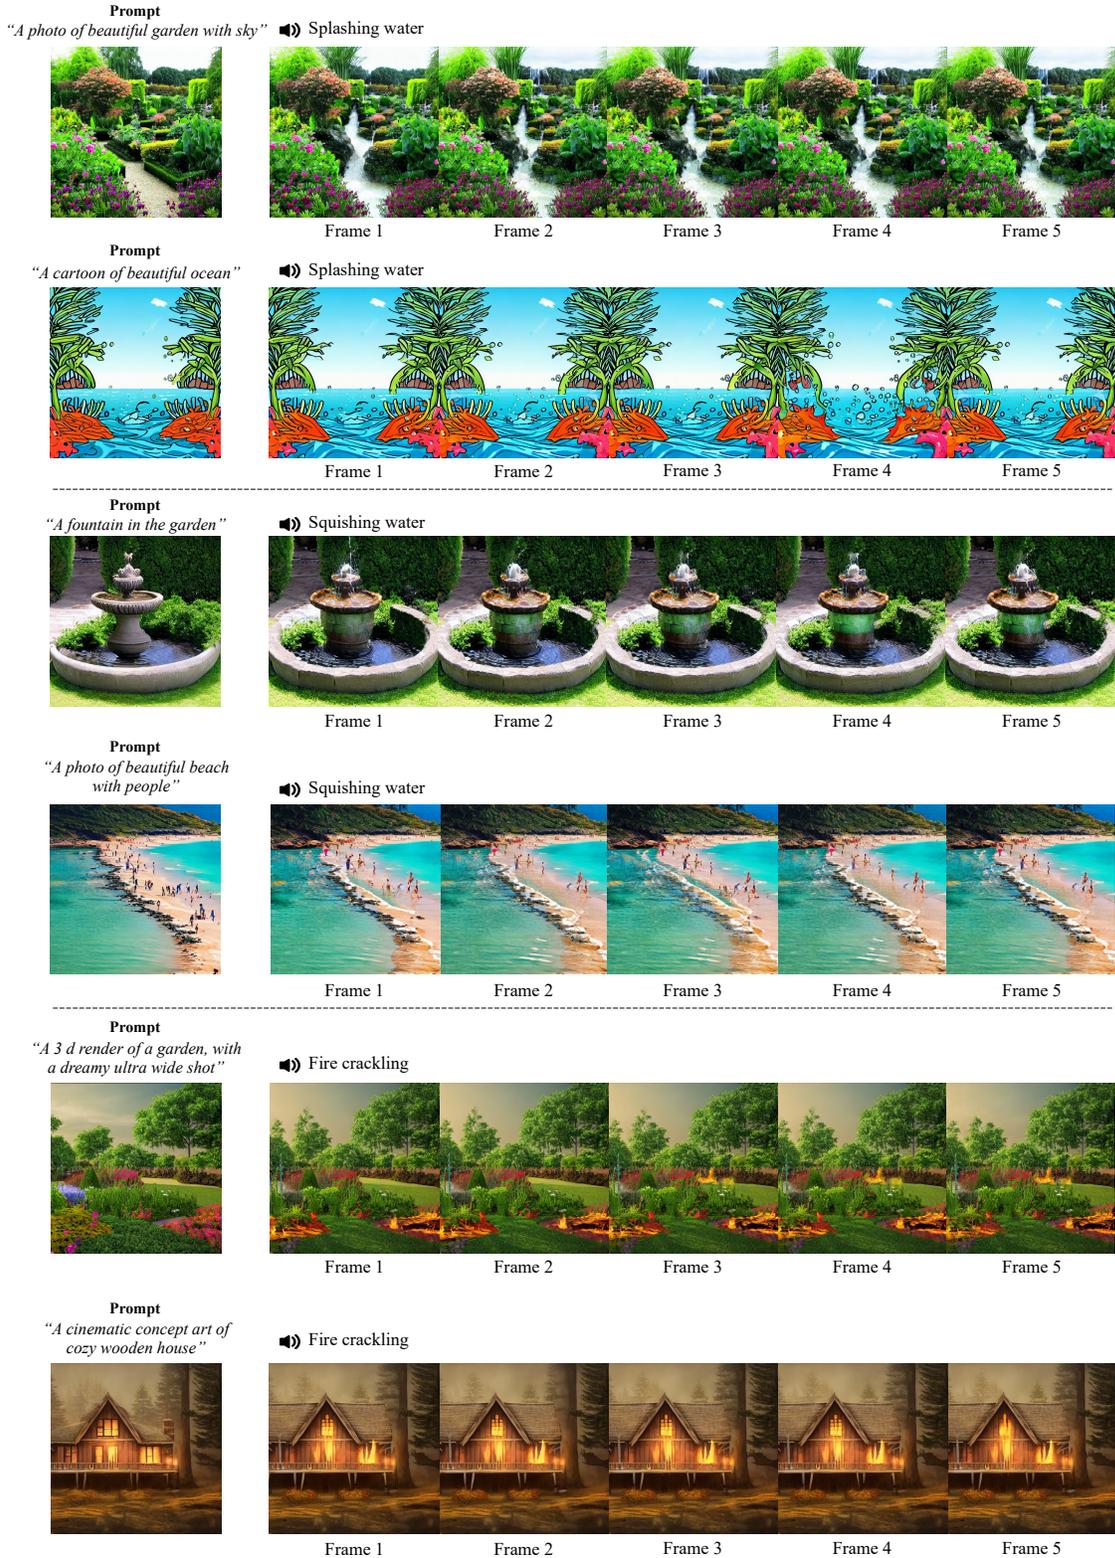

Figure 2: Examples of diverse examples in open domains. The sound of splashing water, squishing water and fire crackling are used.

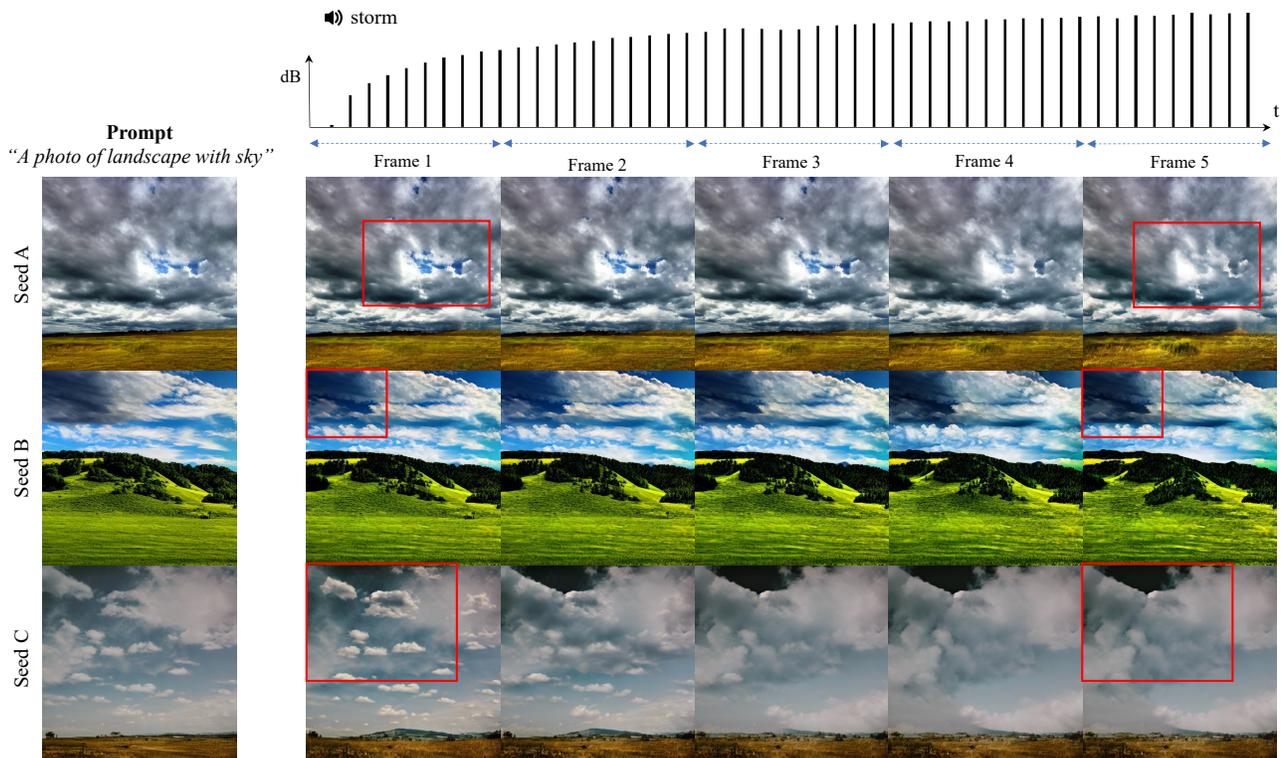

Figure 3: Example of video frames with multiple seed numbers. We regulate the prompt and audio sound as a given input feature and change a seed number randomly. The video frames are temporally consistent with the magnitude of audio.

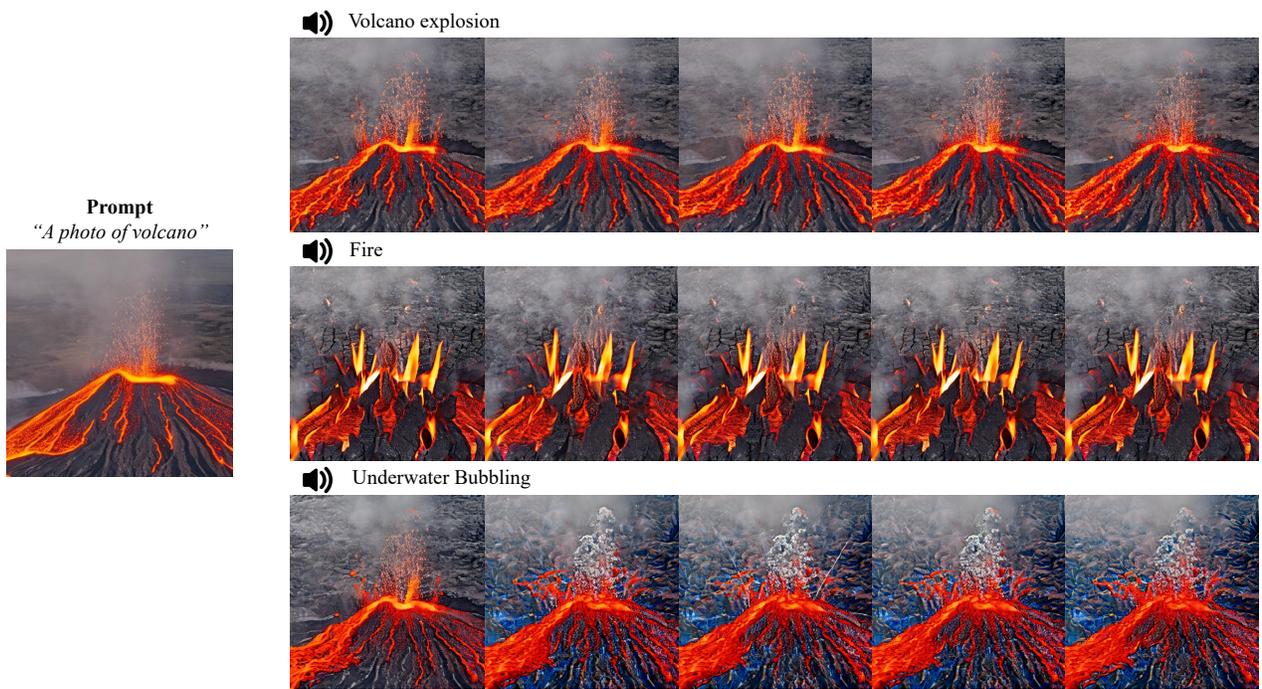

Figure 4: Example of video frames with different sound. The video frames are consistent and relevant with the audio semantics.

Prompt: "A photo of firewood in the forset"

🔊 Fire crackling

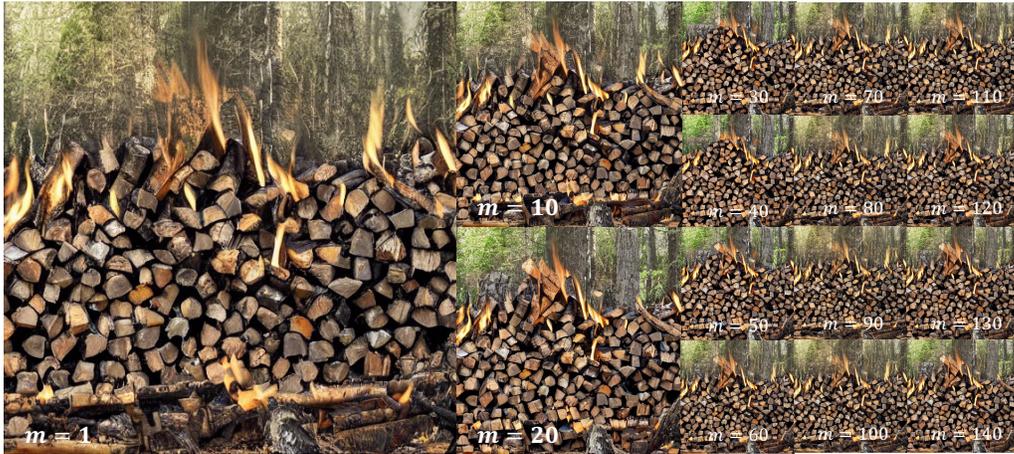

Prompt: "A photo of beautiful park with sky"

🔊 Rain → Bird singing (sunny weather)

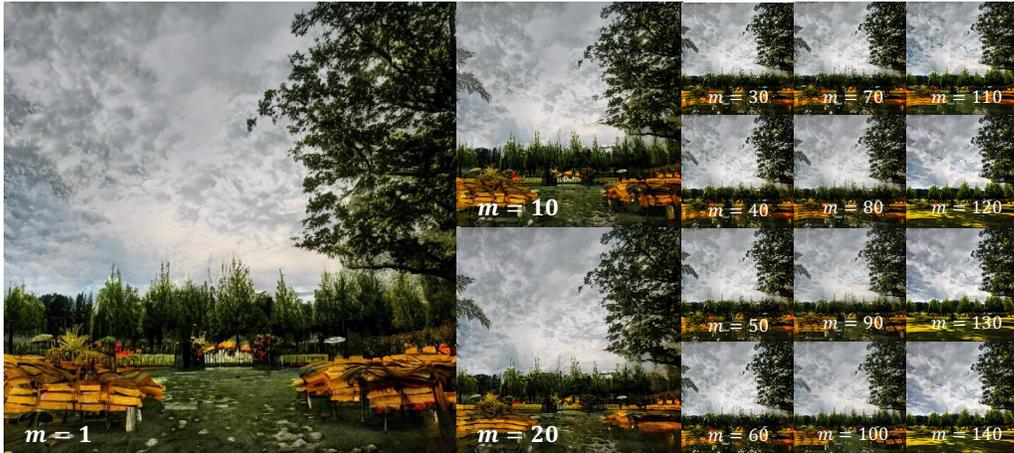

Prompt: "A photo of volcano"

🔊 explosion

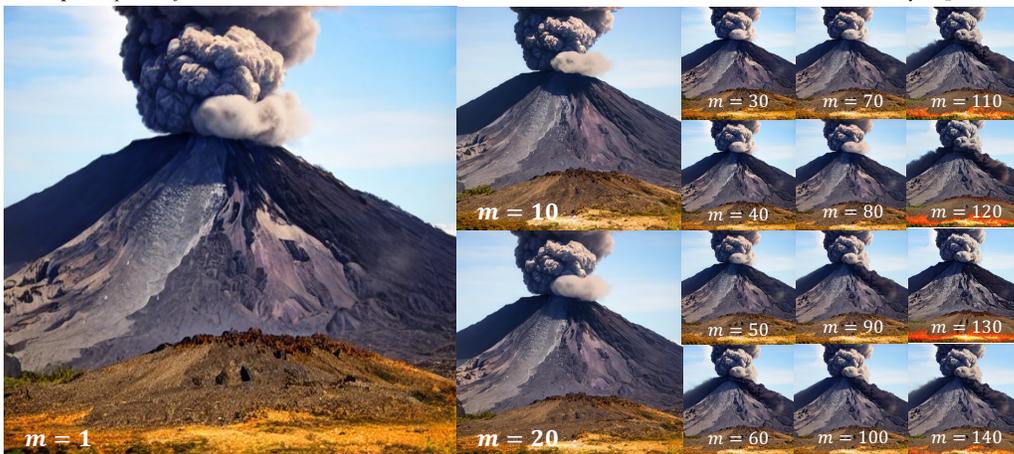

Figure 5: Example of video frames with interpolation module. A number of video frames are generated reactively by audio sound.

## References

- [1] Manuel Brack, Patrick Schramowski, Felix Friedrich, Dominik Hintersdorf, and Kristian Kersting. The stable artist: Steering semantics in diffusion latent space. *arXiv preprint arXiv:2212.06013*, 2022. [1](#)
- [2] Moitrey Chatterjee and Anoop Cherian. Sound2sight: Generating visual dynamics from sound and context. In *Computer Vision–ECCV 2020: 16th European Conference, Glasgow, UK, August 23–28, 2020, Proceedings, Part XXVII 16*, pages 701–719. Springer, 2020. [2](#)
- [3] Honglie Chen, Weidi Xie, Andrea Vedaldi, and Andrew Zisserman. Vggsound: A large-scale audio-visual dataset. In *ICASSP 2020-2020 IEEE International Conference on Acoustics, Speech and Signal Processing (ICASSP)*, pages 721–725. IEEE, 2020. [1](#)
- [4] Dasaem Jeong, Seungheon Doh, and Taegyun Kwon. Träumerai: Dreaming music with stylegan. *arXiv preprint arXiv:2102.04680*, 2(4):10, 2021. [2](#)
- [5] Tero Karras, Miika Aittala, Samuli Laine, Erik Härkönen, Janne Hellsten, Jaakko Lehtinen, and Timo Aila. Alias-free generative adversarial networks. *Advances in Neural Information Processing Systems*, 34:852–863, 2021. [1](#), [2](#)
- [6] Diederik P Kingma and Jimmy Ba. Adam: A method for stochastic optimization. *arXiv preprint arXiv:1412.6980*, 2014. [1](#)
- [7] Seung Hyun Lee, Gyeongrok Oh, Wonmin Byeon, Chanyoung Kim, Won Jeong Ryoo, Sang Ho Yoon, Hyunjun Cho, Jihyun Bae, Jinkyu Kim, and Sangpil Kim. Sound-guided semantic video generation. In *Computer Vision–ECCV 2022: 17th European Conference, Tel Aviv, Israel, October 23–27, 2022, Proceedings, Part XVII*, pages 34–50. Springer, 2022. [1](#), [2](#)
- [8] Alec Radford, Jong Wook Kim, Chris Hallacy, Aditya Ramesh, Gabriel Goh, Sandhini Agarwal, Girish Sastry, Amanda Askell, Pamela Mishkin, Jack Clark, et al. Learning transferable visual models from natural language supervision. In *International conference on machine learning*, pages 8748–8763. PMLR, 2021. [1](#)
- [9] Robin Rombach, Andreas Blattmann, Dominik Lorenz, Patrick Esser, and Björn Ommer. High-resolution image synthesis with latent diffusion models. In *Proceedings of the IEEE/CVF Conference on Computer Vision and Pattern Recognition*, pages 10684–10695, 2022. [1](#)
- [10] Sebastian Ruder. An overview of gradient descent optimization algorithms. *arXiv preprint arXiv:1609.04747*, 2016. [1](#)
- [11] Ivan Skorokhodov, Sergey Tulyakov, and Mohamed Elhoseiny. Stylegan-v: A continuous video generator with the price, image quality and perks of stylegan2. In *Proceedings of the IEEE/CVF Conference on Computer Vision and Pattern Recognition*, pages 3626–3636, 2022. [2](#)
